# Supplementary material for: Quantum Anomalous Hall Effect through Canted Antiferromagnetism
Source: arXiv:1902.10650 ancillary file (2019-02-27)
Supplement: Supplementary file 1 [file supp.pdf]

# Supplemental Material for "Quantum Anomalous Hall Effect through Canted Antiferromagnetism"

Xiao Li,[1] Allan H. MacDonald,[2] and Hua Chen[3,4]

[1]*Center for Quantum Transport and Thermal Energy Science, School of Physics and Technology, Nanjing Normal University, Nanjing 210023, China*
[2]*Department of Physics, The University of Texas at Austin, Austin, TX 78712, USA*
[3]*Department of Physics, Colorado State University, Fort Collins, CO 80523, USA*
[4]*School of Advanced Materials Discovery, Colorado State University, Fort Collins, CO 80523, USA*

## I. FIELD-INDUCED SPIN-FLOP TRANSITION IN $NiF_2$

### A. Spin-flop transition in $NiF_2$ based on a classical spin model

Spin-flop transition usually refers to field-induced rotation of the Néel order parameter in collinear antiferromagnets. In the absence of spin-orbit coupling or magnetocrystalline anistropy, the Néel vector prefers to be perpendicular to the magnetic field, since there is a small but nonzero energy gain

$$\delta E = -2g\mu_B SH\sin\theta + 2NJS^2\sin^2\theta \approx -2g\mu_B SH\theta + 2NJS^2\theta^2, \tag{1}$$

where $\theta$ is a small canting angle induced by the magnetic field, $N$ is the number of nearest neighbors in the other magnetic sublattice, $J$ is the antiferromagnetic exchange coupling. In equilibrium one can get $\theta$ by minimizing Eq. 1, which gives

$$\theta = \frac{g\mu_B H}{2NJS}. \tag{2}$$

Substituting this into Eq. 1 one can get

$$\delta E = -\frac{(g\mu_B H)^2}{2NJ} < 0 \tag{3}$$

which is a second order effect. This is expected since when $H = 0$ the total magnetization vanishes in a Néel antiferromagnet. In the absence of magnetic anisotropy the spin-flop transition occurs for arbitrarily small fields. In reality the energy gain on the order of Eq. 3 must overcome the energy cost of anisotropy for the transition to happen.

In $NiF_2$ the single-ion anisotropy leads to a nonzero net magnetization which can couple to the magnetic field directly. On the other hand, the size of the net magnetization will not be constant when the sublattice moments rotate away from the ground state configuration. Therefore one cannot describe the problem of field-induced rotation of a weak ferromagnet as that for a real ferromagnet with very small but fixed size local moments, where the effect of magnetic field is simply to compete with the single-ion anisotropy. Below we use the model by Moriya[1] and the approach proposed in our previous work[2] to discuss the field-induced coherent rotation of $NiF_2$ moments.

Moriya's model for a single magnetic unit cell of $NiF_2$ is

$$\mathcal{H} = 4J_1\boldsymbol{S}_1\cdot\boldsymbol{S}_2 + \frac{D}{2}(S_{1z}^2 + S_{2z}^2) - \frac{E}{2}[(S_{1x}^2 - S_{1y}^2) - (S_{2x}^2 - S_{2y}^2)], \tag{4}$$

where $1, 2$ label two magnetic sublattices, $J_1 > 0$ is the nearest neighbor antiferromagnetic coupling, $D > 0$ is an easy-plane anisotropy, and $E > 0$ is a small in-plane anisotropy, which tries to maximize $S_{1x}$ and $S_{2y}$. Thus a nonzero $E$ leads to finite canting of the local spins.

We consider the limit of $J_1 \gg D \gg E$, for which the lowest energy configuration has $S_{1z} = S_{2z} = 0$, i.e., the moments are within the $xy$ plane. We can then represent $S_{ix}$ and $S_{iy}$ by the azimuthal angle $\phi_i$ of the $i$-th moment:

$$S_{ix} = S\cos\phi_i,\ \ S_{iy} = S\sin\phi_i. \tag{5}$$

Eq. 4 thus becomes

$$\begin{aligned}\mathcal{H} &= 4J_1S^2(\cos\phi_1\cos\phi_2 + \sin\phi_1\sin\phi_2) - \frac{1}{2}ES^2(\cos^2\phi_1 - \sin^2\phi_1 - \cos^2\phi_2 + \sin^2\phi_2) \\ &= 4J_1S^2\cos(\phi_1-\phi_2) + ES^2\sin(\phi_1+\phi_2)\sin(\phi_1-\phi_2) \\ &\equiv 4J_1S^2\cos\phi_A + ES^2\sin\phi_S\sin\phi_A.\end{aligned} \tag{6}$$

Taking derivatives of this $\mathcal{H}$ with respect to $\phi_A = \phi_1 - \phi_2$ and $\phi_S = \phi_1 + \phi_2$, we arrive at two equations

$$\begin{aligned}&-4J_1S^2\sin\phi_A + ES^2\sin\phi_S\cos\phi_A = 0, \\ &ES^2\cos\phi_S\sin\phi_A = 0.\end{aligned} \tag{7}$$

The solution of above equations is

$$\begin{aligned}&\phi_S = (n+\frac{1}{2})\pi,\ \ n\in Z, \\ &\phi_A = (-1)^n\arctan\frac{E}{4J_1} + m\pi \approx (-1)^n\frac{E}{4J_1} + m\pi,\ \ m\in Z.\end{aligned} \tag{8}$$

However, not all solutions correspond to energy minima. To see this we substitute Eq. 8 into Eq. 6, which gives

$$\mathcal{H} = 4J_1S^2(-1)^m \cos\frac{E}{4J_1} + ES^2(-1)^m \sin\frac{E}{4J_1}. \tag{9}$$

Thus for minimal H $m$ can only be odd integers, while no constraint is placed on $n$. The solutions for $\phi_1$ and $\phi_2$ are therefore

$$\begin{aligned}\phi_1 &= (-1)^n\frac{E}{8J_1} + \left(\frac{n}{2} + m + \frac{3}{4}\right)\pi, \\ \phi_2 &= (-1)^{n+1}\frac{E}{8J_1} + \left(\frac{n}{2} - m - \frac{1}{4}\right)\pi,\end{aligned} \tag{10}$$

where we have replaced $m$ by $2m+1$ so that $m$ can be arbitrary integers.

By trying different values of $m$ and $n$, one can find that there are four inequivalent solutions:

$$\begin{aligned}(\phi_1,\phi_2) = (\phi_0 - \frac{\pi}{4}, -\phi_0 + \frac{3\pi}{4}),\ (\phi_0 + \frac{3\pi}{4}, -\phi_0 - \frac{\pi}{4}), \\ (-\phi_0 + \frac{\pi}{4}, \phi_0 + \frac{5\pi}{4}),\ (-\phi_0 + \frac{5\pi}{4}, \phi_0 + \frac{\pi}{4}),\end{aligned} \tag{11}$$

where $\phi_0 \equiv E/8J_1$ is the canting angle. The two solutions in each line are mutually time-reversal partners, while the two lines differ by a $\pi/2$ rotation plus $\phi_0 \to -\phi_0$. In other words, there are four energy minima corresponding to the weak magnetization pointing to four in-plane directions separated by integer multiples of $\pi/2$.

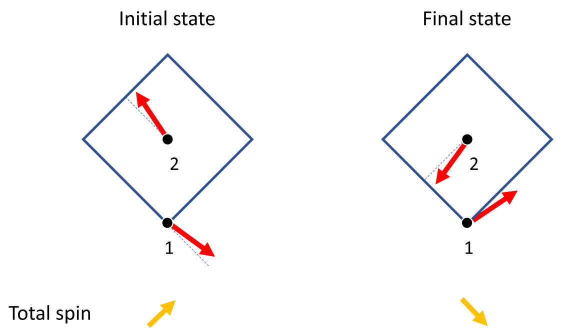


FIG. 1. Initial and final states considered in the rotation. One can notice that the spin on site 1 rotates counterclockwisely by less than 90 degrees while that on site 2 rotates by more than 90 degrees, making the net spin effectively rotates clockwisely by 90 degrees.

We expect $\phi_s \equiv (\phi_1 + \phi_2)/2$ characterizes the rigid rotation of the order parameter while $\phi_a \equiv (\phi_1 - \phi_2)/2$ changes little through the rotation process. We take the first column of Eq. 11 as the initial and final states (Fig. 1), i.e.

$$(\phi_s, \phi_a) = (\frac{\pi}{4}, \phi_0 - \frac{\pi}{2}),\ (\frac{3\pi}{4}, -\phi_0 - \frac{\pi}{2}) \tag{12}$$

The total spin is given by

$$\begin{aligned}(S_x, S_y) &= S(\cos\phi_1 + \cos\phi_2, \sin\phi_1 + \sin\phi_2) \\ &= 2S(\cos\phi_s\cos\phi_a, \sin\phi_s\cos\phi_a),\end{aligned} \tag{13}$$

according to which the net spins for the initial and final states are respectively

$$(S_x, S_y)_{i,f} = \sqrt{2}S\sin\phi_0(1, \pm 1). \tag{14}$$

To make the final state lower in energy the magnetic field must be along $-\hat{x} + \hat{y}$ direction, i.e., opposite to that of $\boldsymbol{S}_f$ because of the negative g-factor. The Zeeman term thus becomes

$$\begin{aligned}\mathcal{H}_z &= -\frac{g\mu_B H}{\sqrt{2}}[(S_{1x} + S_{2x}) - (S_{1y} + S_{2y})] \\ &= -2g\mu_B HS\cos\phi_a\cos(\phi_s + \frac{\pi}{4}).\end{aligned} \tag{15}$$

Thus for $\boldsymbol{S}_f$ $H_z = -2g\mu_B HS\sin\phi_0$ which is negative.

The Hamiltonian we would like to minimize is therefore

$$\mathcal{H} = 4J_1S^2\cos(2\phi_a) + ES^2\sin(2\phi_s)\sin(2\phi_a) - 2g\mu_B HS\cos\phi_a\cos(\phi_s + \frac{\pi}{4}). \tag{16}$$

To make the problem simpler we consider the ranges of $\phi_s$ and $\phi_a$ in the switching process. Since $\phi_s$ starts from $\pi/4$ and ends at $3\pi/4$, we can redefine $\phi_s$ by

$$\phi_s = \psi_s + \frac{\pi}{4}, \tag{17}$$

so that

$$\begin{cases} \psi_s \in [0, \pi/2], & \text{counterclockwise rotation} \\ \psi_s \in [0, -3\pi/2], & \text{clockwise rotation} \end{cases} \tag{18}$$

Similarly, since $\phi_a$ changes from $\phi_0 - \pi/2$ to $-\phi_0 - \pi/2$, we redefine it by

$$\phi_a = \psi_a - \frac{\pi}{2}, \tag{19}$$

so that $\psi_a$ is a small angle. Eq. 16 can be written using $\psi_{s,a}$ as

$$\mathcal{H} = -4J_1S^2\cos(2\psi_a) - ES^2\cos(2\psi_s)\sin(2\psi_a) + 2g\mu_B HS\sin\psi_a\sin\psi_s. \tag{20}$$

The balance equations are now

$$\begin{cases} 8J_1S^2\sin(2\psi_a) - 2ES^2\cos(2\psi_s)\cos(2\psi_a) + 2g\mu_B HS\cos\psi_a\sin\psi_s = 0 \\ 2ES^2\sin(2\psi_s)\sin(2\psi_a) + 2g\mu_B HS\sin\psi_a\cos\psi_s = 0 \end{cases} \tag{21}$$

If we further assume $\psi_a \ll 1$ which is reasonable, we arrive at the following two equations

$$\begin{cases} \psi_a = \frac{E}{8J_1}\cos(2\psi_s) - \frac{g\mu_B H}{8J_1S}\sin\psi_s \\ \psi_a\cos\psi_s(4ES\sin\psi_s + g\mu_B H) = 0 \end{cases} \tag{22}$$

From the 2nd equation we can get three possibilities: $\psi_a = 0$, $\cos\psi_s = 0$, or $\sin\psi_s = -g\mu_B H/4ES$. They correspond to different extrema along the rotation path, which we have solved and listed in Table I.

TABLE I. Energy extrema along the rotation path.

| | $\psi_s$ | $\psi_a$ |
|---|---|---|
| Global minimum (final state) | $\frac{\pi}{2}$ | $-\phi_0\left(1+\frac{H}{H_a}\right)$ |
| Local minimum (TR of final state) | $-\frac{\pi}{2}$ | $-\phi_0\left(1-\frac{H}{H_a}\right)$ |
| Local minima (initial state and its TR) | $\sin\psi_s = -\frac{H}{4H_a}$ | $\phi_0\left(1+\frac{H^2}{8H_a^2}\right)$ |
| Maxima | Eq. 23 | 0 |

Fig. 2 shows the $\psi_s$ values of the different extrema depending on the magnetic field strength. One can see clearly that the initial state moves away from the expected final state, and merges with its original time-reversal partner when $H = 4H_a$. However, from now the system will be trapped at this state since it becomes a local minimum when $H > 4H_a$, and the remaining two local maxima sitting in between it and the desired final state can never merge with it according to the following expressions for the maxima:

$$\sin\psi_s = \begin{cases} -\frac{H}{4H_a} \pm \sqrt{\left(\frac{H}{4H_a}\right)^2 + \frac{1}{2}}, & 0 \le \frac{H}{H_a} \le 1, \\ -\frac{H}{4H_a} + \sqrt{\left(\frac{H}{4H_a}\right)^2 + \frac{1}{2}}, & \frac{H}{H_a} > 1 \end{cases} \tag{23}$$

Separately, these behaviors can also be captured by the evolution of the energy profile versus $H/H_a$. This can be obtained by substituting the first equation in Eq. 22 into the Hamiltonian Eq. 20 and plotting the latter vs. $\psi_s$. Such plots are shown in Fig. 3, from which one can see the initial clockwise rotation (top panel), merging of the two local

maxima with the local minimum at $\psi_s = -\pi/2$ (middle panel), and the trapping of the system at $\psi_s = -\pi/2$ (bottom panel).

Based on these results, if one accepts the model in Eq. 4, with Zeeman coupling only, ignores temperature-assisted transition and stays in the quasi-static limit by increasing magnetic field slowly, deterministic $\pi/2$ rotation of the $NiF_2$ weak magnetization to the field direction can never occur. One can also see that the $\pi$ rotation by using a magnetic field applied in the direction opposite to the initial weak magnetization is not possible.

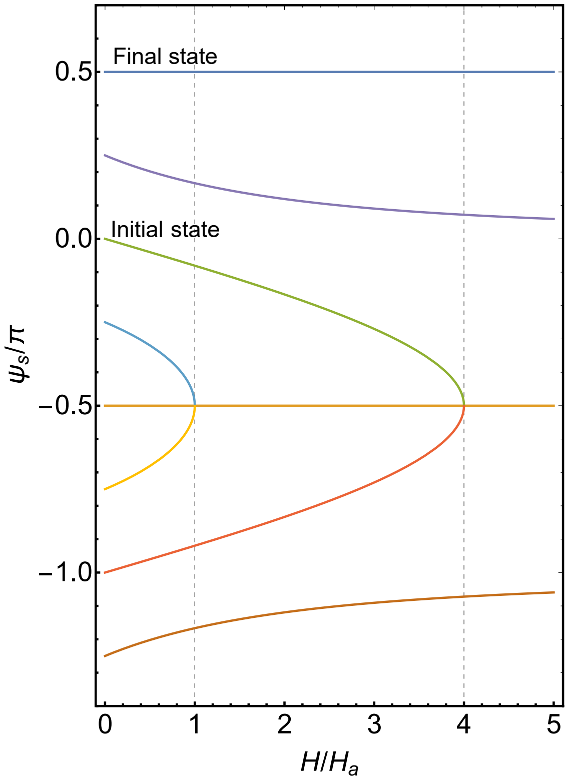


FIG. 2. Dependence of $\psi_s$ of the extrema on $H/H_a$.

To see the underlying reason for this counterintuitive result, we temporarily ignore the external magnetic field, and study the dependence of canting on $\psi_s$. This can be described by dropping the 2nd term on the right hand side of the 1st equation in Eq. 22, i.e.,

$$\psi_a = \frac{E}{8J_1}\cos(2\psi_s). \tag{24}$$

We have studied the same rotation problem under the assumption that the field does not lead to additional canting, and found the $\psi_s$ vs. $H$ plot is qualitatively the same as Fig. 2 for small $H$, and still cannot lead to switching to the desired final state at large $H$. The net spin can now be written as a function of $\psi_s$ only using Eq. 13:

$$\boldsymbol{S}_{tot} = 4S\phi_0\cos(2\psi_s)[\cos(\psi_s + \frac{\pi}{4}), \sin(\psi_s + \frac{\pi}{4})]. \tag{25}$$

$\boldsymbol{S}_{tot}(\psi_s)$ is plotted in Fig. 4, from which one can see that although after $\psi_s$ changes by $\pi/2$ the direction of $\boldsymbol{S}_{tot}$ changes by $\pi/2$, as expected from Fig. 1, at small values of $\psi_s$ $\boldsymbol{S}_{tot}$ still rotates in the same way as the local moments. This leads to the initial clockwise rotation of the local spins that makes them move away from the desired final state and finally trapped in the rotation path. However, as we will show below, the orbital magnetization has a very different angular dependence from that in Fig. 4, which provides a remedy for the pathological switching behavior.

### B. Effect of orbital magnetization

To qualitatively capture the behavior of the orbital magnetization in the structure of $NiF_2$, we construct a minimal $s-d$ model by considering a single $s$-electron hopping between Ni sites in the $NiF_2$ structure, with opposite, in-plane

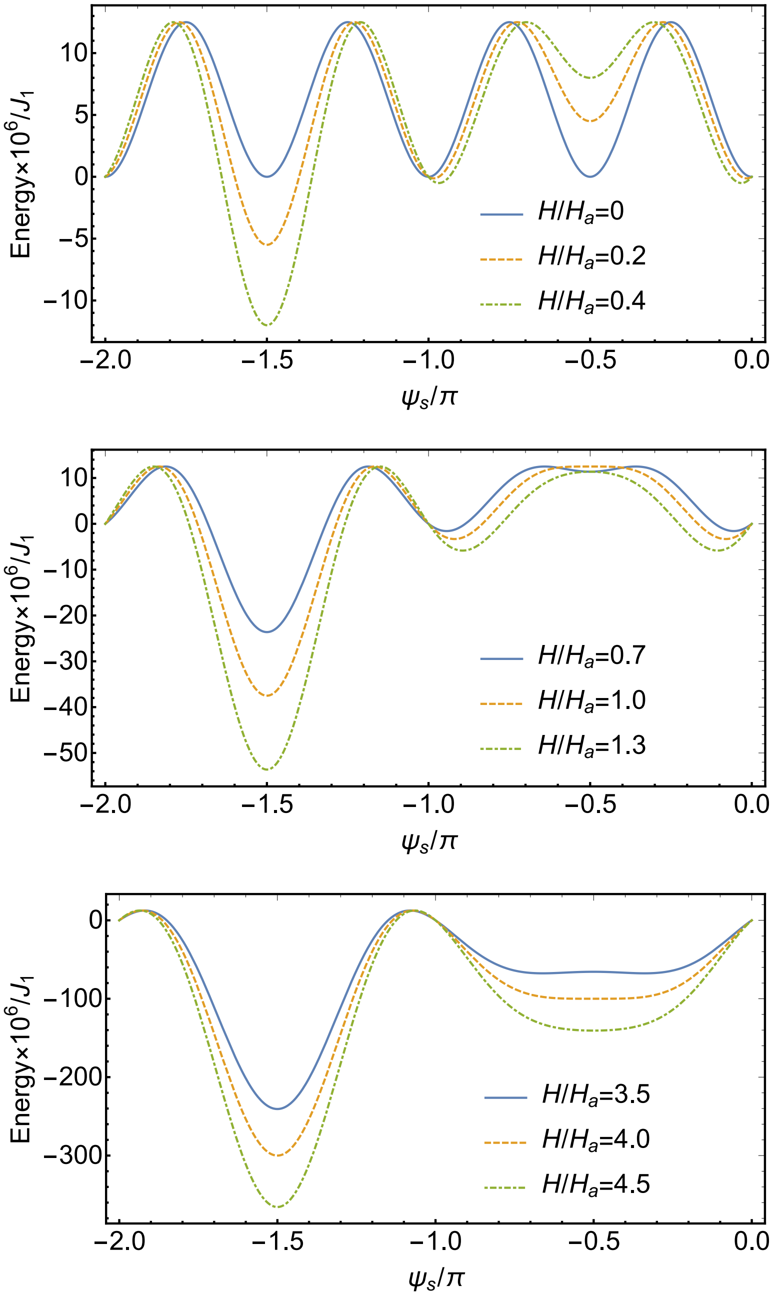


FIG. 3. Dependence of the energy profile on $H/H_a$. $E/J_1 = 0.01$. The ground state energy when $H = 0$ is set to zero energy.

exchange fields on the two Ni sublattices, and a spin-orbit coupling term allowed by the symmetry of $NiF_2$. The Hamiltonian is written as

$$\begin{aligned} H &= H_t + H_{ex} + H_{so} \\ &= -t_1 \sum_{\langle i\alpha, j\beta\rangle_1 \gamma} c^\dagger_{i\alpha\gamma} c_{j\beta\gamma} - t_2 \sum_{\langle ij\rangle_2 \alpha\gamma} c^\dagger_{i\alpha\gamma} c_{j\alpha\gamma} - t_3 \sum_{\langle ij\rangle_3 \alpha\gamma} c^\dagger_{i\alpha\gamma} c_{j\alpha\gamma} \\ &\quad - \sum_{i\alpha\gamma\delta} J_{ex} (\hat{n}_\alpha \cdot \boldsymbol{\sigma}_{\gamma\delta}) c^\dagger_{i\alpha\gamma} c_{i\alpha\delta} \\ &\quad + \mathrm{i}\lambda_{so} \sum_{\langle i\alpha, j\beta\rangle_1 \gamma} [(\hat{\eta}_{i\alpha, j\beta} \times \hat{r}_{i\alpha, j\beta}) \cdot \boldsymbol{\sigma}_{\gamma\delta}] c^\dagger_{i\alpha\gamma} c_{j\beta\gamma}, \end{aligned} \tag{26}$$

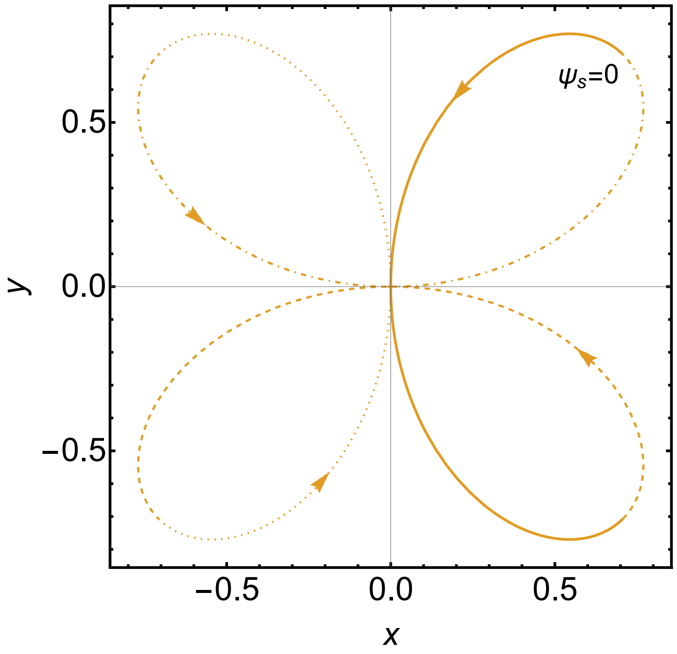


FIG. 4. Angular dependence of the total spin due to anisotropy-induced canting with $\psi_s$ increasing from 0 to $2\pi$. Solid, dashed, dotted, and dot-dashed lines respectively correspond to $\psi_s \in [0, \pi/2]$, $[\pi/2, \pi]$, $[\pi, 3\pi/2]$, $[3\pi/2, 2\pi]$.

where $i, j$ label unit cell, $\alpha, \beta$ label sublattices, and $\gamma, \delta$ label spin. $t_{1,2,3}$ are the strengths of hopping along different paths. $t_1$ is the hopping along the gray bonds shown in Fig. 5, $t_2$ is that between nearest neighbors along $c$-axis, and $t_3$ is that between nearest neighbors along $a$- or $b$-axis. $J_{ex}$ is the strength of the on-site exchange fields, whose directions are along $\hat{n}_\alpha$. $\lambda_{so}$ is the spin-orbit coupling strength. $\hat{r}_{i\alpha,j\beta}$ is a unit vector pointing from site $i\alpha$ to site $j\beta$, and $\hat{\eta}_{i\alpha,j\beta}$ are unit vectors indicated by the arrows in Fig. 5. The spin-orbit coupling term is written down using the method described in the main text, but can be understood as due to the F atoms close to each Ni-Ni bond shown in the figure which break the inversion symmetry with respect to the bond centers.

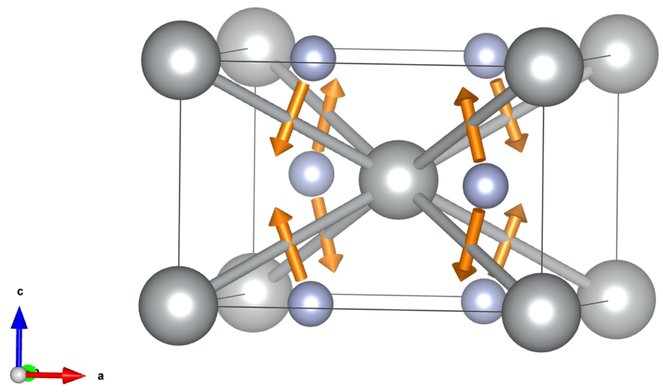


FIG. 5. Spin-orbit coupling vectors in the s-d model, based on the inversion-symmetry-breaking Ni-Ni bonds in $NiF_2$.

Similar to the $s-d$ model for $Mn_3Ir$, the present model can give a nonzero intrinsic anomalous Hall conductivity when the Fermi energy is not within the band gap, even if the exchange fields on the two sublattices are exactly antiparallel with each other. When the Fermi energy is within the band gap, integration of the Berry curvature over the filled bands within the 3D Brillouin zone vanishes, but one can still obtain a nonzero orbital magnetization. Fig. 6 shows the dependence of the orbital magnetization on $\psi_s$ by setting $\psi_a = 0$. Here $\psi_s$ and $\psi_a$ describe the directions of the local exchange fields, $n_\alpha$. Surprisingly, compared to Fig. 4 for the canting-induced total spin in the

phenomenological model, the orbital magnetization behaves much more regularly with increasing $\psi_s$. Specifically, the orbital magnetization simply rotates oppositely to the local exchange fields throughout $\psi_s \in [0, 2\pi)$, and there are no nodes where the orbital magnetization vanishes. For the switching process considered above, if the dominant coupling to the external magnetic field is through the orbital magnetization, the local spins will consistently rotate clockwisely to maximize this coupling until the system reaches the final state.

The appearance of the nodes in Fig. 4 is actually an artifact of the classical spin model. Note that the nodes appear when one sublattice spin is parallel to the local in-plane easy axis while the other is perpendicular to the local easy axis. When this happens canting cannot further reduce the energy, which leads to perfect cancellation of the two spins. However, that the two spins always have the same length is an artificial constraint of the model. Since at this special angle the two sites are not equivalent from symmetry point of view, they do not necessarily have the same local spin density. In addition, even if the two sublattices spins can be assumed to be of the same length, it is not necessary that their g-factors are the same and isotropic. In particular, the nonzero orbital magnetization at $\psi_s = \pi/4$ can be viewed as an effect of unequal g-factors of the two sublattice spins at this angle. We would therefore like to make the comment that if one were to describe orbital-dominated AHE AFMs with phenomenological Heisenberg-type models, the effective g-tensor would be strongly dependent on order parameter direction.

The artificial constraint of the classical spin model also leads to the more complicated angular dependence of the total spin compared to that of the orbital magnetization. One could represent the in-plane components of the total spin by the real and imaginary parts of a complex function of $\psi_s$, and expand it into Fourier series of $\psi_s$. The lowest order Fourier component that can capture the opposite rotations of the total spin vs. sublattice spins by only considering the four equivalent minima is proportional to $e^{-i\psi_s}$. However, such a Fourier component alone cannot lead to the nodes at $\psi_s = (2n+1)\pi/4$, $n$ being any integer, which requires another Fourier component, $e^{3i\psi_s}$, to be of the same weight as $e^{-i\psi_s}$ in the series (Eq. 25). Discarding this artificial constraint allows $e^{-i\psi_s}$ to appear by itself as the lowest-order Fourier component, which is exactly what Fig. 6 shows for the case of orbital magnetization.

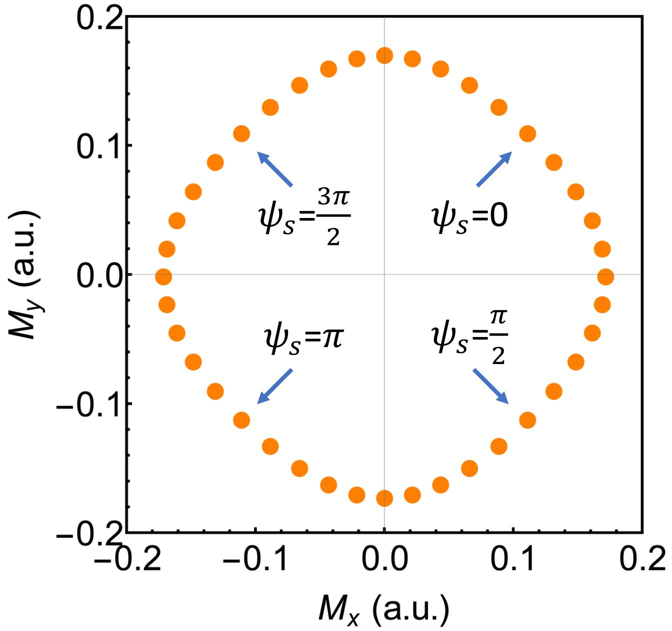


FIG. 6. Dependence of the in-plane components of the orbital magnetization on rotation angles of the local exchange fields $\psi_s$. Points corresponding to $\psi_s = n\pi/2$ are indicated by arrows. Note that increasing $\psi_s$ means counterclockwise rotation of the local exchange fields, while the orbital magnetization rotates clockwisely.

## II. MINIMAL MODEL FOR THE STRUCTURE OF HEMATITE

The hematite has a rhombohedral structure with four Fe atoms per unit cell 7, and has the $D_{3d}^6$ symmetry[3]. We denote the four Fe atoms in Fig. 7, from top to bottom, as Fe1, Fe2, Fe3, and Fe4. In the high-temperature phase (state II) between 250 K and 950 K, the directions of the four Fe moments satisfy $\boldsymbol{M}_{Fe1} = -\boldsymbol{M}_{Fe2} = -\boldsymbol{M}_{Fe3} = \boldsymbol{M}_{Fe4}$, and they are all perpendicular to the (111) axis, which is also a trigonal axis.

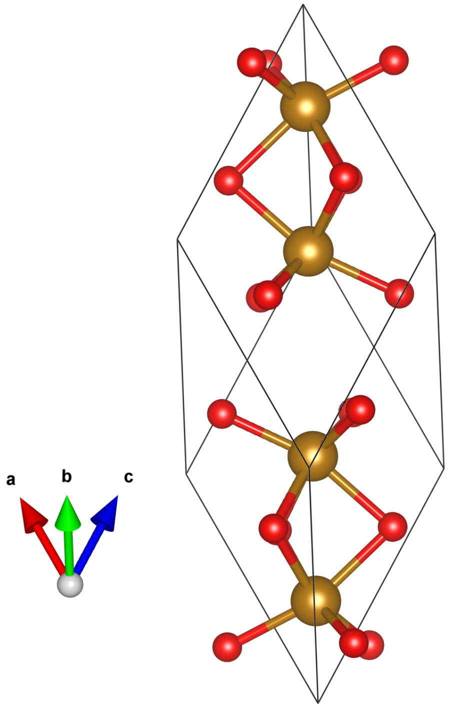


FIG. 7. Unit cell of $\alpha{-}Fe_2O_3$ (hematite).

The weak ferromagnetism in hematite, as it is now well known, is due to the Dzyaloshinskii-Moriya interaction. The Dzyaloshinskii-Moriya interaction (DMI) between two spins $\boldsymbol{S}_1$ and $\boldsymbol{S}_2$ has the form of $\boldsymbol{D} \cdot (\boldsymbol{S}_1 \times \boldsymbol{S}_2)$. Since interchanging 1 and 2 changes the sign of $\boldsymbol{S}_1 \times \boldsymbol{S}_2$ while energy must be a scalar, it follows that $\boldsymbol{D}$ is not invariant under space inversion with respect to the center of the bond between 1 and 2. Namely, there must be inversion symmetry breaking with respect to the center of a bond between to spins for the Dzyaloshinskii-Moriya interaction to be nonzero. This argument is somewhat reminiscent of the way we wrote the spin-orbit coupling terms in the s-d models for $Mn_3X$ and $NiF_2$. Indeed, for a nearest neighbor bond similar to that in $Mn_3X$ and $NiF_2$, the inversion symmetry breaking at the bond center is characterized by a single polar vector $\hat{\eta}_{12}$ (Fig. 5), and one can therefore define two mutually perpendicular mirror planes going through the bond center and parallel with the polar vector. Based on the general rule that this energy term must be invariant under these symmetry operations, one can find that $\boldsymbol{D}$ must be parallel with the mirror that is perpendicular to the bond, but perpendicular to the mirror that is parallel with the bond. Thus we must have $\boldsymbol{D} \parallel \hat{r}_{12} \times \hat{\eta}_{12}$. This is the reason why the DMI vector due to the inversion symmetry breaking at the surface of a ferromagnet is always parallel to the surface.

The case of hematite is, however, a little more complicated than this. There is a $C_3$ symmetry with respect to the (111) axis. Therefore for the bond between Fe1 and Fe2, for example, one cannot define a $\hat{\eta}$ that has components perpendicular to (111). Such a type of inversion symmetry breaking makes our naive strategy of constructing $s-d$ models not applicable, since one cannot write down a spin-orbit coupling of the form in Eq. 26. However, we can go back to the basics and consider the origin of the spin-orbit coupling:

$$H_{so} = \lambda_{so} (\nabla V \times \boldsymbol{p}) \cdot \boldsymbol{s}. \tag{27}$$

the spin-orbit coupling in the s-d model is basically writing this term in the $s$-orbital basis. In this case $\langle s|\nabla V|s\rangle$ is a simple constant vector, and because of the cross product with $\boldsymbol{b}$ only its projection to the plane normal to $\boldsymbol{b}$ is relevant. However, if there is a larger than 2-fold rotation symmetry with respect to $\boldsymbol{b}$, such as the Fe1-Fe2 bond in the case of hematite, $\langle s|\nabla V|s\rangle$ must not have any component perpendicular to $\boldsymbol{b}$, which is the reason why we cannot write a spin-orbit coupling term in the $s-d$ model. Nonetheless, it is not necessarily so for the matrix elements of $\nabla V$ in the $p$-orbital basis, or any basis with $> 1$ dimensionality.

To find the expression of $\nabla V$ in the $p$-orbital basis, we note that it should be a 3-component vector with each component being a $3 \times 3$ matrix. For a Hermitian matrix of dimension $N$ there are $N^2$ independent parameters. Thus in the $p$-orbital basis $\nabla V$ has $3 \times 3^2 = 27$ independent parameters. In principle they can be fixed if we have

27 independent equations. Since the defining property of $\nabla V$ is the three-fold rotation symmetry with respect to the bond between Fe1 and Fe2, we next show how a vector operator in the $p$-orbital basis rotates.

For a scalar operator in the $p$-orbital basis, it rotates in exactly the same way as a rank-2 tensor, since $|p_x\rangle$, $|p_y\rangle$ and $|p_z\rangle$ transforms as $x$, $y$, $z$ under rotation:

$$p_\alpha \equiv \langle r|p_\alpha\rangle = \sqrt{\frac{3}{4\pi}}\frac{\alpha}{r},\ \alpha = x,\ y,\ z. \tag{28}$$

Thus a rotation operator in the $p$-orbital basis looks identical to its expression in the Cartesian coordinate basis $(x, y, z)$. If we denote an arbitrary rotation matrix as $R_{\boldsymbol{\theta}}$, where $\boldsymbol{\theta} = \theta\hat{n}$ means rotating around the unit vector $\hat{n}$ by an angle $\theta$, a scalar operator in the $p$-orbital basis rotates as

$$O' = R_{\boldsymbol{\theta}} O' R_{\boldsymbol{\theta}}^T, \tag{29}$$

since $R_{\boldsymbol{\theta}}^T = R_{\boldsymbol{\theta}}^\dagger = R_{\boldsymbol{\theta}}^{-1}$.

For a vector operator $\hat{\boldsymbol{O}}$, the rotation not only modifies each of its three components through Eq. 29, but will also change the three components as a vector, which means that

$$O'_i = \sum_j (R_{\boldsymbol{\theta}})_{ij}(R_{\boldsymbol{\theta}} O_j R_{\boldsymbol{\theta}}^T). \tag{30}$$

Eq. 30 leads to an interesting conclusion. If we denote $\langle p_i|\hat{O}_k|p_j\rangle$ as $O_{ijk}$, we have

$$O'_{lmn} = (R_{\boldsymbol{\theta}})_{li}(R_{\boldsymbol{\theta}})_{mj}(R_{\boldsymbol{\theta}})_{nk} O_{ijk}. \tag{31}$$

Namely, one can simply recognize $O_{ijk}$ as a rank-3 Cartesian tensor.

Above argument can be extended to include other point-group symmetry operations, and one only needs to specify whether the physical quantity corresponding to the vector operator $\hat{\boldsymbol{O}}$ is a polar or pseudo (axial) vector. For the former, $O_{ijk}$ corresponds to a rank-3 polar tensor while for the latter it corresponds to a rank-3 pseudo tensor.

There is a well-established method for getting symmetry-allowed components of arbitrary Cartesian tensors, as detailed in[4]. Above arguments make it clear that we can use this approach to get the desired form of $\nabla V$ in the $p$-orbital basis. Considering the atomic complex formed by the two nearest neighboring Fe atoms and the three O atoms forming a triangle perpendicular to the Fe-Fe bond, the system has a symmetry group of $D_{3h}$ (it is not so if we include further oxygen atoms, but we use this symmetry group here for simplicity), which includes the following 12 elements:

$$E,\ 2C_3,\ \sigma_h,\ 2S_3,\ 3C'_2,\ 3\sigma_v, \tag{32}$$

where $E$ is the unit element, $2C_3$ means two $C_3$ rotations with respect to the Fe-Fe bond (taken as $z$ axis), $\sigma_h$ is the reflection with respect to the mirror perpendicular to the 3-fold axis, $2S_3$ means two 3-fold improper rotations $(C_3 \times \sigma_h)$, $3C'_2$ means three 2-fold rotation axes in the $xy$ plane (prime means these axes are not the same), and $3\sigma_v$ means three mirror planes parallel with the $z$ axis.

By applying the generators of the $D_{3h}$ group onto a rank-3 polar tensor, and by requiring that it is invariant under these symmetry operations, one can eliminate most of the components. Ref.[4] provides a convenient table for the results, which for $D_{3h}$ group and $y$ parallel with one of the three 2-fold axes are

$$\begin{aligned} &O_{xxy} = O_{xyx} = O_{yxx} = -O_{yyy}, \\ &0\,\text{otherwise}. \end{aligned} \tag{33}$$

Thus we arrive at

$$O_x = \begin{pmatrix} 0 & -1 & 0 \\ -1 & 0 & 0 \\ 0 & 0 & 0 \end{pmatrix},\ O_y = \begin{pmatrix} -1 & 0 & 0 \\ 0 & 1 & 0 \\ 0 & 0 & 0 \end{pmatrix},\ O_z = 0_{3\times 3}, \tag{34}$$

where we have absorbed a common scalar coefficient in the $\lambda_{so}$.

We can finally write down the desired spin-orbit coupling matrix in the $p$-orbital basis for the hopping along the positive $z$ direction:

$$\begin{aligned} H_{so} &= i\lambda_{so}(O_x \otimes \sigma_y - O_y \otimes \sigma_x) \\ &= \lambda_{so}\begin{pmatrix} 0 & i & 0 & -1 & 0 & 0 \\ i & 0 & 1 & 0 & 0 & 0 \\ 0 & -1 & 0 & -i & 0 & 0 \\ 1 & 0 & -i & 0 & 0 & 0 \\ 0 & 0 & 0 & 0 & 0 & 0 \\ 0 & 0 & 0 & 0 & 0 & 0 \end{pmatrix}. \end{aligned} \tag{35}$$

To write down the full tight-binding $p-d$ model, we consider the nearest and 2nd nearest Fe-Fe neighbors, which form a network as shown in Fig. 8.

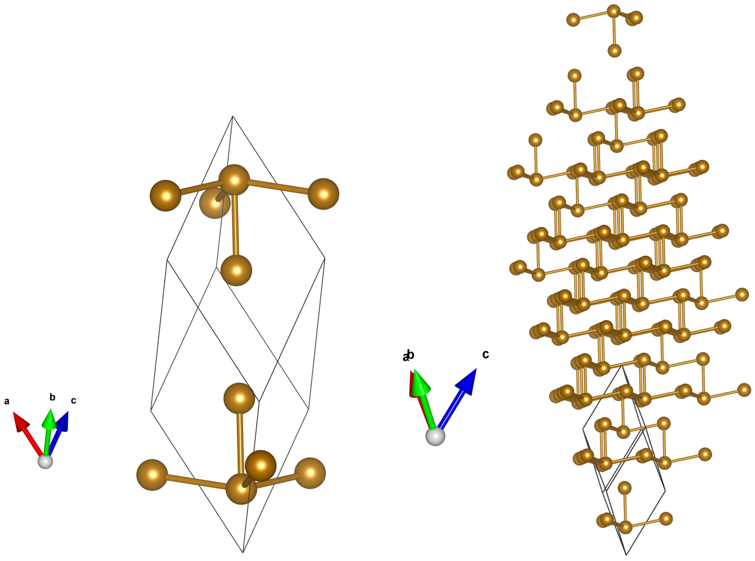


FIG. 8. Fe atoms in hematite with only 1st and 2nd nearest Fe-Fe bonds considered. The right panel shows the 3D network formed by Fe atoms in a larger $(3 \times 3 \times 3)$ cell.

The tight-binding Hamiltonian is then written as

$$H = \sum_{\langle i\alpha, j\beta\rangle_{1,2}\gamma} t_{i\alpha,j\beta} c^\dagger_{i\alpha\gamma} c_{j\beta\gamma} + \sum_{i\langle\alpha,\beta\rangle_1\gamma\delta} \mathrm{i}\lambda_{so} (\boldsymbol{O}_{\alpha\beta} \times \boldsymbol{\sigma}_{\gamma\delta}) \cdot \hat{d}_{\alpha\beta} c^\dagger_{i\alpha\gamma} c_{i\beta\delta} - \sum_{i\alpha\gamma\delta} J \hat{n}_\alpha \cdot \boldsymbol{\sigma}_{\gamma\delta} c^\dagger_{i\alpha\gamma} c_{i\alpha\delta}, \tag{36}$$

where $i, j$ label unit cells, $\alpha, \beta$ label sublattices as well as orbitals on each site, $\gamma\delta$ label spin, $\langle\rangle_{1,2}$ means both nearest and next nearest neighbors, $t_{i\alpha,j\beta}$ is the spin-independent hopping between $p$-orbitals on different sites, $\lambda_{so}$ is the strength of the spin-orbit coupling, $\boldsymbol{O}_{\alpha\beta}$ is the symmetry-restricted matrix for $\nabla V$ as discussed above, $J$ is the strength of a site-dependent exchange field representing the antiferromagnetic order of hematite, and $\hat{n}_\alpha$ is its direction on each sublattice. For simplicity we assume $\hat{n} = \hat{x}$ for Fe1 and Fe4, and $\hat{n} = -\hat{x}$ for Fe2 and Fe3. The magnetically order state thus has inversion symmetry with respect to the center between Fe2 and Fe3.

$t_{i\alpha,j\beta}$ are basically the hopping matrix elements between $p$ orbitals, and are represented by the Slater-Koster parameters:

$$\begin{aligned} E_{x,x} &= l^2 V_{pp\sigma} + (1-l^2) V_{pp\pi} \\ E_{x,y} &= lm V_{pp\sigma} - lm V_{pp\pi} \\ E_{x,z} &= ln V_{pp\sigma} - ln V_{pp\pi}, \end{aligned} \tag{37}$$

where $l, m, n$ are the directional cosines defined as $(l, m, n) = (r_x, r_y, r_z)/r$ for a bond along $\boldsymbol{r}$. The parameters not shown in the table above can be obtained by cyclic permutation of $x, y, z$ together with $l, m, n$. $V_{pp\sigma}$ and $V_{pp\pi}$ are parameters representing the strength of the $\sigma$ bond and the $\pi$ bond for $p$ orbitals, respectively. According to[5] they are

$$\begin{aligned} V_{pp\sigma} &= 3.24 \frac{\hbar^2}{md^2}, \\ V_{pp\pi} &= -0.81 \frac{\hbar^2}{md^2}, \end{aligned} \tag{38}$$

where $d$ is the interatomic distance. Note that $|V_{pp\sigma}| > |V_{pp\pi}|$ at the same distance, as expected. In our toy model we set $V_{pp\sigma}$ at the nearest neighbor distance as the energy unit. The nearest neighbor $V_{pp\pi} = -0.25$. The 2nd nearest neighbor hoppings are parametrized by $V_{pp\sigma} \equiv t_2$ and $V_{pp\pi} = -0.25 t_2$.

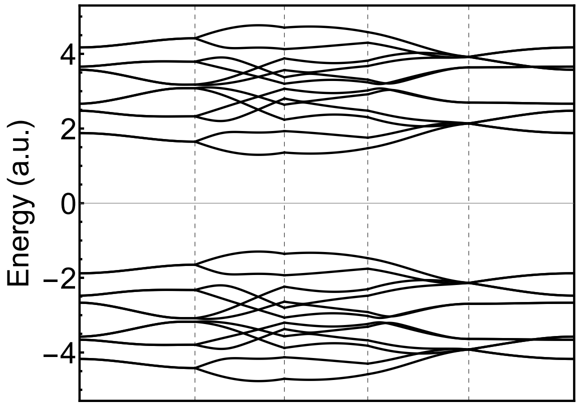


FIG. 9. Band structure of the $p-d$ model having the symmetry of $\alpha-Fe_2O_3$. The parameter values are $t_2 = 0.8$, $\lambda_{so} = 0.3$, and $J = 3$.

For the bond between Fe1 and Fe2, $\boldsymbol{O}_{\alpha\beta}$ takes the form in Eq. 34. The $\boldsymbol{O}_{\alpha\beta}$ for the Fe3-Fe4 bond can be obtained by performing a spatial inversion operation on it, which simply changes its overall sign. This completes our toy model for the hematite structure.

A typical band structure of the model described above is shown in Fig. 9, which has 24 bands. Note that when $J = 0$ the system has both time-reversal and inversion symmetry. The inversion center is the midpoint between Fe2 and Fe3. Due to Kramers theorem all bands should be doubly degenerate, and we find that it is indeed the case. When $J \neq 0$ both the time-reversal symmetry and the inversion symmetry are broken. Their combination is not a good symmetry either. Therefore the bands are not doubly degenerate in general. Another check can be done by flipping the Zeeman fields on Fe3 and Fe4, which makes the combination of time-reversal and inversion a good symmetry, and should lead to doubly degenerate bands. This has also been confirmed using the toy model.

We calculated the orbital magnetization and the anomalous Hall conductivity by setting the Fermi energy to $-4.6$ in the band structure in Fig. 9, and found that they are both nonzero, and are along the $y$ axis as expected.

## III. ON THE PARTICLE-HOLE SYMMETRY OF THE TOY MODEL

The 2D toy model in the main text has an emergent particle-hole symmetry $\mathcal{C} \equiv \tau_z\sigma_y$ which makes

$$\mathcal{C}^\dagger H_{\boldsymbol{k}}\mathcal{C} = -H^T_{-\boldsymbol{k}}, \tag{39}$$

where $T$ means transpose and $H_{\boldsymbol{k}}$ includes all five terms described in the main text. The particle-hole symmetry is reminiscent of Bogoliubov-de Gennes (BdG) Hamiltonians of conventional superconductors which have $\mathcal{C}' = \tau_x \otimes \mathbb{I}$, where $\tau_x$ is in the Nambu spinor space and $\mathbb{I}$ is the identity matrix in the normal state Hilbert space. However, in contrast to $\mathcal{C}'^*\mathcal{C}' = 1$ for the BdG case, we have $\mathcal{C}^*\mathcal{C} = -1$. Gapped non-interacting Hamiltonians with such a particle-hole symmetry and broken time-reversal symmetry belong to class C of the ten-fold Altland-Zirnbauer classification, and in 2D have a $2\mathbb{Z}$ topological invariant[6,7]. Although the particle-hole symmetry here is not as robust as that in BdG Hamiltonians since it can be broken by, e.g., a next-nearest-neighbor hopping, when $\mathcal{C}$ is present the model may be effectively viewed as a class C topological superconductor hosting two chiral "Majorana" edge states. We also mention that other gap terms can be used instead of $H_{\text{cant}}$ to give QAHE, e.g., a spin-independent sublattice potential ($H_\Delta \propto \tau_z\sigma_0$). However, since $H_\Delta$ breaks the $\mathcal{C}$ symmetry we can get a Chern number equal to 1. A possible alternative is a staggered hopping term that breaks inversion symmetry (i.e., similar to $H_\Delta$ but odd under $\boldsymbol{k} \to -\boldsymbol{k}$), which makes the $\mathcal{C}$ symmetry intact but is not as practical as the canting.

[1] T. Moriya, Phys. Rev. **117**, 635 (1960).
[2] Hua Chen, Tzu-Cheng Wang, Di Xiao, Guang-Yu Guo, Qian Niu, and Allan H. MacDonald, arXiv:1802.03044
[3] I. Dzyaloshinskii, J. Phys. Chem. Solids **4**, 241 (1958).

[4] R. R. Birss, *Symmetry and Magnetism* (North-Holland, Amsterdam, 1966).
[5] W. A. Harrison, *Electronic Structure and the Properties of Solids* (Dover, New York, 1989).
[6] S. Ryu, A. P. Schnyder, A. Furusaki, and A. W. W. Ludwig, New J. Phys. **12**, 065010 (2010).
[7] C.-K. Chiu, J. C. Y. Teo, A. P. Schnyder, and S. Ryu, Rev. Mod. Phys. **88**, 035005 (2016).
